# Supplementary material for: Can Large Language Models Be Query Optimizer for Relational Databases?
Source: arXiv:2502.05562 source file (2025-02-08)
Supplement: Supplementary file 1 [file appendix.tex]

\appendix
\twocolumn[
\centerline{\Huge \bfseries Appendix} % Use \Large or another size command as needed for your style
\vspace{\baselineskip} % Provide the vertical space after the title
]

\section*{Additional Experiment of Effectiveness}
Table~\ref{tab:multi} shows the overall performance across different types of graphs on both CS/ACS tasks. We test three pairs of different types of datasets for training and inference, naming X2Y, where X is a dataset for training and Y is a different type of dataset for inference, respectively. The three pairs are \Arxivproduct, \Twitterciteseer, and \Corafacebook.

We summarize our main observations as follows. 
As Table~\ref{tab:multi} illustrates, \IACS surpasses the best baselines in \Fone score of $0.29\%$, $2.33\%$ and $5.80\%$ for \Twitterciteseer, \Arxivproduct and \Corafacebook, respectively. Our \IACS framework outperforms all the baselines when applied to different types of graphs, which verifies that the model can be transferred across different types of graphs effectively. 

In addition, as a further investigation, we  compare the performance of \IACS on the datasets in Table~\ref{tab:nonacs}-\ref{tab:acsmulti} in the paper with the new datasets in Table~\ref{tab:multi}. We observe that the performance advantages of \IACS for different types of datasets are not as significant as those within the same type of datasets or a single dataset. For instance, when compared with the best baselines, our models exhibit an improvement of $3.89\%$ in \Fone score in \Citeseer, $2.12\%$ in \Coraciteseer, and $0.29\%$ in \Twitterciteseer, respectively. For the \Product dataset, our \IACS models achieve a $2.35\%$ improvement compared to the best baselines, and a slightly less improvement ($2.33\%$) for \Arxivproduct.
Moreover, the performance improvement in \Facebook is quite non-trivial, with a $5.69\%$ increment in \Fone scores, while a larger improvement of $8.04\%$ is achieved in \Twitterfacebook. In the case of \Corafacebook, the improvement is still less ($5.80\%$) compared to datasets of the same type. This disparity may be attributed to the relatively limited number of training tasks available for the \Facebook dataset (only 7 tasks). In contrast, in \Twitterfacebook and \Corafacebook, the training tasks are relatively abundant, resulting in more remarkable improvements.

\section*{Efficiency}
Fig.~\ref{fig:timetrainingcomplete} and \ref{fig:timecomplete} present a comprehensive comparison of the GPU training and inference time across all the datasets. The results are consistent with that of Fig.~\ref{fig:time} in the paper. Notably, our \IACS models stand out with the shortest training and inference time among all the methods in ACS tasks.
\IACS only fails to surpass \Featrans for non-attributed CS tasks. The results can be attributed to the fact that \Featrans possesses a simpler architecture, which makes training faster. 

\begin{figure*}
  \centering
  \includegraphics[width=0.6\textwidth]{fig/time_legend_finetuning.pdf}
  \resizebox{0.9\textwidth}{!}{
  \begin{tabular}{c}  
  \subfigure[Non-attributed Community Search]{
    \includegraphics[width=0.31\textwidth]{fig/time_CS_finetuningtraining.pdf}
    \label{fig:CStimetrainingcomplete}
}
 \hspace{-0.2cm}
  \subfigure[Attributed Community Search]{
    \includegraphics[width=0.68\textwidth]{fig/time_ACS_finetuningtraining.pdf}
  \label{fig:ACStimetrainingcomplete}}\\
  \end{tabular}}
   \caption{Overall Comparison of Training Time (Second)}
 \label{fig:timetrainingcomplete}
\end{figure*}

\begin{figure*}
  \centering
  \includegraphics[width=0.45\textwidth]{fig/legend_time.pdf}
  \resizebox{0.9\textwidth}{!}{
  \begin{tabular}{c}  
  \subfigure[Non-attributed Community Search]{
    \includegraphics[width=0.28\textwidth]{fig/time_CS.pdf}
    \label{fig:CStimecomplete}
}
 \hspace{-0.2cm}
  \subfigure[Attributed Community Search]{
    \includegraphics[width=0.62\textwidth]{fig/time_ACS.pdf}
  \label{fig:ACStimecomplete}}\\
  \end{tabular}}
   \caption{Overall Comparison of Inference Time (Second)}
 \label{fig:timecomplete}
\end{figure*}

\begin{table}
\caption{Overall Performance on CS/ACS in Different Types of Graphs (\%)}
\label{tab:multi}
%\vspace{-0.2cm}
\centering
\resizebox{0.5\textwidth}{!}{
\begin{tabular}{c|c|ccc|ccc}
\toprule
\multicolumn{1}{c|}{}                          & \multicolumn{1}{c|}{}          & \multicolumn{3}{c|}{{ 4-shot}} & \multicolumn{3}{c}{{8-shot}} \\%\cline{3-8}
\multicolumn{1}{c|}{\multirow{-2}{*}{Dataset}} & \multicolumn{1}{c|}{\multirow{-2}{*}{Approach}}       & \Pre              & \Rec          & \Fone               & \Pre              & \Rec          & \Fone               \\\midrule
  & \CTC       & $77.44_{\pm0.43}$  & $4.74_{\pm0.30}$  & $8.92_{\pm0.54}$  & $76.77_{\pm0.12}$ & $4.70_{\pm0.18}$  & $8.87_{\pm0.33}$  \\
 & \ICSGNN    & $79.50_{\pm0.22}$  & $6.57_{\pm0.01}$  & $12.14_{\pm0.01}$ & $79.49_{\pm0.35}$ & $6.55_{\pm0.01}$  & $12.10_{\pm0.02}$ \\
 & \QDGNN     & $75.62_{\pm0.18}$ & $95.22_{\pm0.21}$ & $84.30_{\pm0.03}$ & $75.34_{\pm0.35}$ & $96.82_{\pm0.66}$ & $84.74_{\pm0.03}$ \\
 & \Supervise & $84.04_{\pm0.20}$ & $77.22_{\pm0.71}$ & $80.49_{\pm0.29}$ & $84.54_{\pm0.23}$ & $80.45_{\pm0.57}$ & $82.44_{\pm0.18}$ \\
 & \MAML      & $80.19_{\pm0.05}$ & $60.35_{\pm1.89}$  & $68.86_{\pm1.24}$ & $80.80_{\pm0.98}$ & $38.48_{\pm6.05}$ & $51.97_{\pm5.35}$ \\
 & \Featrans  & $78.87_{\pm0.33}$ & $57.50_{\pm0.37}$ & $66.51_{\pm0.13}$  & $79.19_{\pm0.82}$ & $58.13_{\pm0.81}$ & $67.03_{\pm0.24}$ \\\cline{2-8}
 & \IACS      & $78.26_{\pm0.47}$ & $97.02_{\pm0.43}$ & $86.64_{\pm0.13}$  & $79.03_{\pm0.39}$ & $96.43_{\pm0.36}$ & $86.86_{\pm0.09}$ \\
 & \IACSGATE  & $79.06_{\pm0.95}$ & $96.11_{\pm1.08}$ & \underline{${86.75_{\pm0.23}}$} & $79.46_{\pm0.58}$  & $96.10_{\pm0.66}$ & \underline{${86.99_{\pm0.15}}$} \\
\multirow{-9}{*}{\rotatebox{90}\Arxivproduct} & \IACSPLAIN & $79.13_{\pm0.86}$ & $96.15_{\pm0.77}$ & \cellcolor{LightCyan}{$\mathbf{86.81_{\pm0.25}}$} & $79.26_{\pm0.91}$ & $96.63_{\pm0.79}$ & \cellcolor{LightCyan}{$\mathbf{87.08_{\pm0.23}}$}

\\ \midrule
& \ATC       & $57.81_{\pm1.17}$ & $5.11_{\pm0.32}$  & $9.39_{\pm0.55}$  & $57.96_{\pm2.24}$ & $5.01_{\pm0.36}$  & $9.21_{\pm0.64}$  \\
 & \ACQ       & $69.32_{\pm1.72}$  & $7.06_{\pm1.29}$   & $12.78_{\pm2.09}$ & $69.88_{\pm0.81}$ & $6.83_{\pm1.16}$  & $12.43_{\pm1.91}$  \\
 & \AQDGNN    & $50.42_{\pm0.72}$  & $72.80_{\pm2.59}$ & $59.56_{\pm0.37}$ & $51.19_{\pm1.78}$ & $82.51_{\pm5.90}$  & $63.17_{\pm3.07}$ \\
 & \Supervise & $58.26_{\pm0.77}$ & $61.03_{\pm0.26}$ & $59.61_{\pm0.28}$  & $61.90_{\pm1.39}$ & $65.61_{\pm1.36}$ & $63.71_{\pm1.38}$ \\
 & \MAML      & $55.83_{\pm1.13}$ & $49.35_{\pm4.01}$ & $52.34_{\pm2.59}$ & $57.98_{\pm2.80}$  & $54.48_{\pm8.34}$  & $56.09_{\pm5.75}$ \\
 & \Featrans  & $53.70_{\pm1.33}$ & $57.04_{\pm1.77}$ & $55.32_{\pm1.45}$ & $53.15_{\pm2.76}$ & $60.56_{\pm4.62}$ & $56.45_{\pm1.22}$ \\\cline{2-8}
 & \IACS      & $59.14_{\pm3.00}$ & $60.74_{\pm2.68}$ & $59.84_{\pm0.85}$  & $60.81_{\pm2.90}$ & $67.47_{\pm4.21}$ & $63.85_{\pm1.72}$ \\
 & \IACSGATE  & $60.20_{\pm0.29}$ & $59.41_{\pm3.01}$ & \underline{${59.87_{\pm1.41}}$} & $62.66_{\pm3.39}$  & $65.92_{\pm3.39}$ & {\cellcolor{LightCyan}$\mathbf{64.12_{\pm1.16}}$} \\
\multirow{-9}{*}{\rotatebox{90}\Twitterciteseer} & \IACSPLAIN & $60.23_{\pm1.04}$ & ${60.10_{\pm3.15}}$ & \cellcolor{LightCyan}{$\mathbf{60.12_{\pm1.36}}$} & $62.07_{\pm2.99}$ & $65.86_{\pm1.61}$ & \underline{$63.88_{\pm2.06}$}

\\ \midrule
& \ATC       & $72.54_{\pm3.57}$ & $15.07_{\pm4.80}$ & $24.71_{\pm6.37}$ & $76.20_{\pm5.43}$  & $11.34_{\pm1.73}$ & $19.69_{\pm2.67}$ \\
 & \ACQ       & $7.72_{\pm0.36}$ & $62.81_{\pm0.86}$ & $13.76_{\pm0.55}$ & $19.12_{\pm1.82}$ & $49.54_{\pm5.85}$ & $27.59_{\pm2.78}$ \\
 & \AQDGNN    & $36.12_{\pm1.02}$ & $96.59_{\pm3.69}$ & $52.56_{\pm1.28}$ & $36.42_{\pm1.04}$ & $93.99_{\pm7.48}$  & $52.47_{\pm2.26}$ \\
 & \Supervise & $56.99_{\pm3.67}$  & $81.78_{\pm1.98}$ & $67.08_{\pm1.92}$ & $61.34_{\pm4.33}$ & $79.65_{\pm8.65}$ & $69.23_{\pm5.62}$ \\
 & \MAML      & $52.67_{\pm1.81}$ & $65.50_{\pm2.52}$ & $58.35_{\pm0.12}$ & $53.03_{\pm7.31}$ & $88.47_{\pm1.33}$  & $66.13_{\pm5.35}$  \\
 & \Featrans  & $38.80_{\pm3.29}$ & $85.94_{\pm7.73}$ & $53.32_{\pm3.40}$ & $35.06_{\pm2.16}$  & $71.24_{\pm3.97}$ & $47.00_{\pm2.80}$ \\\cline{2-8}
 & \IACS      & $64.29_{\pm3.13}$  & $85.39_{\pm3.46}$  & \underline{$73.25_{\pm1.19}$}  & $65.71_{\pm3.85}$ & $83.90_{\pm4.38}$  & $73.60_{\pm0.73}$ \\
 & \IACSGATE  & $69.87_{\pm2.49}$    & $79.45_{\pm2.49}$ & \cellcolor{LightCyan}$\mathbf{74.30_{\pm0.77}}$  & $65.13_{\pm0.99}$ & $88.34_{\pm0.51}$ & \cellcolor{LightCyan}{$\mathbf{74.98_{\pm0.85}}$} \\
\multirow{-9}{*}{\rotatebox{90}\Corafacebook} & \IACSPLAIN & $65.34_{\pm4.78}$  & $83.35_{\pm6.31}$ & {$72.98_{\pm0.33}$} & $67.22_{\pm1.55}$ & $83.81_{\pm0.11}$ & \underline{$74.60_{\pm0.92}$}
      \\\bottomrule 
\end{tabular}
}
\end{table}
